# Supplementary material for: Deep Movement Primitives: toward Breast Cancer Examination Robot
Source: arXiv:2202.09265 source file (2022-02-14)
Supplement: Supplementary file 1 [file aaai22_apndx.tex]

\relax
\documentclass[letterpaper]{article} % DO NOT CHANGE THIS
\usepackage{aaai22}  % DO NOT CHANGE THIS
\usepackage{times}  % DO NOT CHANGE THIS
\usepackage{helvet}  % DO NOT CHANGE THIS
\usepackage{courier}  % DO NOT CHANGE THIS
\usepackage[hyphens]{url}  % DO NOT CHANGE THIS
\usepackage{graphicx} % DO NOT CHANGE THIS
\urlstyle{rm} % DO NOT CHANGE THIS
  % DO NOT CHANGE THIS
\usepackage{natbib}  % DO NOT CHANGE THIS AND DO NOT ADD ANY OPTIONS TO IT
\usepackage{caption} % DO NOT CHANGE THIS AND DO NOT ADD ANY OPTIONS TO IT
\DeclareCaptionStyle{ruled}{labelfont=normalfont,labelsep=colon,strut=off} % DO NOT CHANGE THIS
\usepackage{subcaption}
\frenchspacing  % DO NOT CHANGE THIS
\setlength{\pdfpagewidth}{8.5in}  % DO NOT CHANGE THIS
\setlength{\pdfpageheight}{11in}  % DO NOT CHANGE THIS
\usepackage{algorithm}
\usepackage{algorithmic}
\usepackage{amssymb}
\usepackage{amsmath}
\usepackage{amsfonts}
\usepackage{booktabs}
\usepackage{threeparttable}
\usepackage{multirow}
\usepackage{rotating}
\usepackage[left=.45in,right=.45in,top=.6in,bottom=.6in,headheight=14.5pt]{geometry}
\usepackage{array,multirow,textcomp}
\usepackage[T1]{fontenc}

\newcolumntype{L}[1]{>{\raggedright\let\newline\\\arraybackslash\hspace{0pt}}m{#1}}
%\newcolumntype{R}[1]{>{\raggedleft\let\newline\\\arraybackslash\hspace{0pt}}m{#1}}
%\newcolumntype{C}[1]{>{\centering\arraybackslash}p{#1}}
\newcolumntype{C}[1]{>{\centering\let\newline\\\arraybackslash\hspace{0pt}}m{#1}}

\setcounter{secnumdepth}{0} %May be changed to 1 or 2 if section numbers are desired.

% Title

% Your title must be in mixed case, not sentence case.
% That means all verbs (including short verbs like be, is, using,and go),
% nouns, adverbs, adjectives should be capitalized, including both words in hyphenated terms, while
% articles, conjunctions, and prepositions are lower case unless they
% directly follow a colon or long dash
\title{Deep Movement Primitives: toward Breast Cancer Examination Robot}
\author{
    Oluwatoyin Sanni,\textsuperscript{\rm 1,*}
    Giorgio Bonvicini,\textsuperscript{\rm 2}
    Muhammad Arshad Khan,\textsuperscript{\rm 1}
    Pablo C. L\'opez-Custodio,\textsuperscript{\rm 1}
    Kiyanoush Nazari,\textsuperscript{\rm 1}
    Amir M. Ghalamzan E.\textsuperscript{\rm 1,}\footnote{Authors contributed equally.} % \\
    % {\normalfont ${^1}$ University of Lincoln, UK,  ${^2}$Politecnico di Milano, Italy}\\ % {\normalfont }
}
\affiliations {
    % Affiliations
    \textsuperscript{\rm 1} University of Lincoln, UK, 
    \textsuperscript{\rm 2} Polytechnic University of Milan, Italy\\
    aghalamzanesfahani@lincon.ac.uk
}
 
% PDF Info Is REQUIRED.
% For /Author, add all authors within the parentheses,
% separated by commas. No accents or commands.
% For /Title, add Title in Mixed Case.
% No accents or commands. Retain the parentheses.
\pdfinfo{
/Title (Deep Movement Primitives: toward Breast Cancer Examination Robot)
/Author (Oluwatoyin Sanni, Giorgio Bonvicini, Muhammad Arshad Khan, Pablo C. Lopez-Custodio, Kiyanoush Nazari, Amir M. Ghalamzan E.)
}

\begin{document}

\maketitle

\renewcommand{\thefigure}{A.\arabic{figure}}
\renewcommand{\thetable}{A.\arabic{table}}
\setcounter{figure}{0}
\setcounter{table}{0}

\section{Appendix}

This appendix supplements the content of the main manuscript. This Appendix includes more details about our Reach-to-palpate (RTP) mock study, the results of the trajectory generated by our proposed Deep Movement Primitives (deep MP), and details about the architecture and results of deep Dynamic movement primitives \cite{ridge2020training, pervez2017learning}

This Appendix has the following sections: (1) Data collection-- namely RTP-RGB dataset used  that is for our mock study; (ii) RTP-RGBD (presented and discussed in the main manuscript); (iii) WPP dataset and a detailed description of the 10 different Ablation studies that we have conducted on the all 10 WPP dataset (\textbf{WPP4} and \textbf{WPP9} were presented and discussed in the main manuscript); (2) The lessons we learned from the RTP-RGB dataset and corresponding mock study; (3) d-DMP implementation details; (4) the performance of deep MP on the 10 WPP experiments. We also presented a higher resolution schematic of the proposed architecture, the trajectories generated by deep MP and a 3D image of the trajectories in the Cartesian space. 

\begin{figure}[tb!]
\centering
\begin{subfigure}[b]{1.0\linewidth}
    \includegraphics[width=1.0\linewidth]{figures/AAAI-phantom config.png}
    \caption{{\small RTP-RGB}}
    \label{fig:configs_rtpgrgb}
\end{subfigure}\\

\begin{subfigure}[b]{1.0\linewidth}
    \includegraphics[width=1.0\linewidth]{figures/phantom config rtprgbd.png}
    \caption{{\small RTP-RGBD}}
    \label{fig:configs_rtpgrgbd}
\end{subfigure}
\caption{{\small Some samples out of the different positions and orientations of the Phantom (a) RTP-RGB dataset, and (b) RTP-RGBD dataset. All the images are taken at robot home configuration shown in Fig. 1b in the paper. The red circle shows the starting point where the robot was brought.}}
\end{figure}

\subsection{Data collection procedure and dataset}
The experimental setup used to collect our data is described in the main content of the paper, in the "Hardware setup and data collection" section.

\begin{figure}[tb!]
    \centering
    \includegraphics[width=.65\linewidth]{figures/robot_setup3.png}
    \caption{{\small 7-DOF Panda arm during RTP-RGB data collection. The Xela sensor reaches to touch the corner of the breast phantom.}}
    \label{fig:setup}
\end{figure}
%<<<<<<< FIG >>>>>>>>>

\paragraph{Reach-to-palpate mock dataset (RTP-RGB)} For the RTP task, our first data collection was a mock dataset, called RTP-RGB, which contains 500 samples. At home position, an RGB image of the phantom was taken by the Realsense camera and afterwards, the Robot end-effector was kinesthetically moved by an Operator to the corner of the Phantom as shown in Fig.~\ref{fig:configs_rtpgrgb}. In summary, our dataset consists of 500 RGB images taken at different phantom positions on the plane and the joints positions during the Kinesthetic demonstration. 
Since the robot movement was executed by a human operator kinesthetically moving the end effector, different trajectories have different lengths and a certain variance in the path followed. The results of this study led us to create another dataset discussed in the next section. Our study is elaborated in the next section.

\begin{table*}[tb!]
\centering
\begin{threeparttable}[b]
\begin{tabular}{@{}ccccccccccc@{}}
\toprule
 && \multicolumn{4}{c}{MSE$^*$} && \multicolumn{4}{c}{Absolute Error$^{**}$} \\
\cmidrule{3-6} \cmidrule{8-11} && Reg. 1 & Reg. 2 & Reg. 3 & Reg. 4 && Reg. 1 & Reg. 2 & Reg. 3 & Reg. 4 \\
\midrule
CNN && \textbf{0.0108} & 0.0176 & 0.0130 & 0.0188 && \textbf{39.7}& 49.6& 36.0& 98.7 \\
FC &&  \textbf{0.0118}& 0.0176 & 0.0137 & 0.0210 && \textbf{46.8}& 51.4& 50.9& 111.5\\
\bottomrule
\end{tabular}
\begin{tablenotes}\footnotesize
\item[*] MSE in radians${}^2$; $^{**}$ Absolute error in mm
\end{tablenotes}
\end{threeparttable}
\caption{{\small Evaluation of RTP models with Average MSE (AveMSE) of the joint trajectory and Average Euclidean Distance (AveED) for the last point of the trajectory in task space for each region of RTP-RGB data set.}}
\label{tab:rtprgb_mse_ed}
\end{table*}

\begin{table}[tb!]
\centering
\begin{threeparttable}[b]
\begin{tabular}{ @{}c@{\hskip 0.7cm}cccc@{} }
\toprule
   & X & Y & Z \\
\midrule
Config I & 0.608& 0.063& 0.086 \\
Config II & 0.516& 0.120& 0.096 \\
Config III & 0.575& 0.015& 0.093 \\
Config IV & 0.488& 0.014& 0.092 \\
\bottomrule
\end{tabular}
\begin{tablenotes}\footnotesize
\item[*] Position in meters
\end{tablenotes}
\end{threeparttable}
\caption{{ \small The position of the breast phantom in robot base frame for configuration I, II, III, IV shown in Figure 5 of main paper. }}
\label{table:wpp_configpos}
\end{table}

\paragraph{Mock study using RTP-RGB dataset}
We used deep MP to learn the RTP task: Fig.~\ref{fig:schem_dpromp} shows a higher resolution schematic than the one presented in the main manuscript.
The results obtained using the RTP-RGB dataset (Table~\ref{tab:rtprgb_mse_ed}) suggests that: (1) we need a more structured dataset to better understand the impact of samples density on the results (Fig.~\ref{fig:xy_ee_final_rtprgb} shows the distribution of the final point of the trajectories in the XY plane); (2) the depth data may be relevant; (3) a more challenging task is needed to showcase the effectiveness of our proposed approach.

\begin{figure}[tb!]
\centering
\begin{subfigure}[b]{0.9\linewidth}
    \includegraphics[width=1.0\linewidth]{figures/2D xy circle.png}
    \caption{{\small RTP-RGB}}
    \label{fig:xy_ee_final_rtprgb}
\end{subfigure} \\

\begin{subfigure}[b]{0.9\linewidth}
    \includegraphics[width=1.0\linewidth]{figures/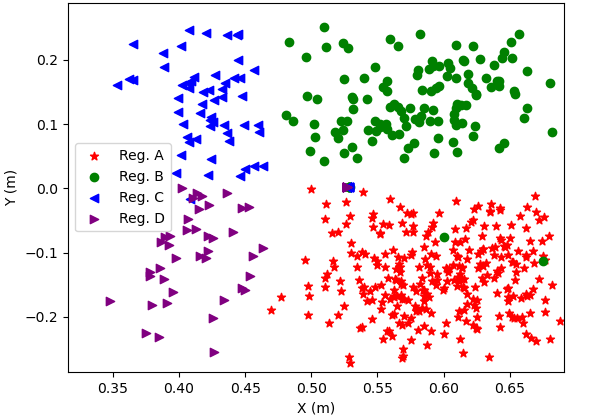}
    \caption{{\small RTP-RGBD}}
    \label{fig:xy_ee_final_rtprgbd}
\end{subfigure}\\
\caption{{\small XY coordinates of the end-effector when the robot reaches the start point of the palpation in RTP-RGB dataset (a) as shown in Fig.~\ref{fig:configs_rtpgrgb} and in RTP-RGBD dataset (b) as shown in Fig.~\ref{fig:configs_rtpgrgbd}. This dataset shows a high variance among the different regions.}}
\end{figure}

\paragraph{Reach-to-palpate final dataset (RTP-RGBD)}
To address the high variance problem in the RTP-RGB mock dataset, we developed the new improved dataset, called RTP-RGBD. This dataset is similar to the previous one, with some exceptions: both RGB and depth images were taken from the robot home position. Also, the reaching movement was not performed by a human operator with Kinesthetic teaching but by the robot, using a regular joint space trajectory and providing the position of the nipple in joint space. This led to a much reduced variance in the trajectory shapes.
Dataset RTP-RGBD was also collected by carefully considering the distribution of the final points of the trajectory on the XY plane. As it can be seen in Fig.~\ref{fig:xy_ee_final_rtprgbd} four regions (named A to D) were defined and samples were collected so that each region had a uniform distribution of points with a different density. The total number of samples in this dataset is 545 with 292, 128, 73 and 52 samples in region A, B, C and D respectively.

\begin{table*}[tb!]
\centering
\begin{tabular}{@{}clccccccc@{}}
\toprule
\multirow{2}{*}{Experiments} && \multicolumn{7}{c}{Palpation patterns} \\
\cmidrule{3-9}  && 1 & 2 & 3 & 4 & 5 & 6 & 7 \\ \midrule
WPP1 && Train & Train & Train & Test & Test & Train & Train \\ \midrule
WPP2 && Train & Train & Test & Test & Train & Train & Train \\ \midrule
WPP3 && Train & Train & Test & Test & Train & Not used & Not used \\ \midrule
\textbf{WPP4} && Train & Test & Test & Train & Train & Not used & Not used \\ \midrule
WPP5 && Train & Train & Train & \begin{tabular}[c]{@{}c@{}}50\% Train\\ 50\% Test\end{tabular} & \begin{tabular}[c]{@{}c@{}}50\% Train\\ 50\% Test\end{tabular} & Train & Train \\ \midrule
WPP6 && Train & Train & \begin{tabular}[c]{@{}c@{}}50\% Train\\ 50\% Test\end{tabular} & \begin{tabular}[c]{@{}c@{}}50\% Train\\ 50\% Test\end{tabular} & Train & Train & Train \\ \midrule
WPP7 && Train & Train & \begin{tabular}[c]{@{}c@{}}50\% Train\\ 50\% Test\end{tabular} & \begin{tabular}[c]{@{}c@{}}50\% Train\\ 50\% Test\end{tabular} & Train & Not used & Not used \\ \midrule
WPP8 && Train & \begin{tabular}[c]{@{}c@{}}50\% Train\\ 50\% Test\end{tabular} & \begin{tabular}[c]{@{}c@{}}50\% Train\\ 50\% Test\end{tabular} & Train & Train & Not used & Not used \\ \midrule
\textbf{WPP9} && \begin{tabular}[c]{@{}c@{}}50\% Train\\ 50\% Test\end{tabular} & \begin{tabular}[c]{@{}c@{}}50\% Train\\ 50\% Test\end{tabular} & \begin{tabular}[c]{@{}c@{}}50\% Train\\ 50\% Test\end{tabular} & \begin{tabular}[c]{@{}c@{}}50\% Train\\ 50\% Test\end{tabular} & \begin{tabular}[c]{@{}c@{}}50\% Train\\ 50\% Test\end{tabular} & \begin{tabular}[c]{@{}c@{}}50\% Train\\ 50\% Test\end{tabular} & \begin{tabular}[c]{@{}c@{}}50\% Train\\ 50\% Test\end{tabular} \\ \midrule
WPP10 && \begin{tabular}[c]{@{}c@{}}50\% Train\\ 50\% Test\end{tabular} & \begin{tabular}[c]{@{}c@{}}50\% Train\\ 50\% Test\end{tabular} & \begin{tabular}[c]{@{}c@{}}50\% Train\\ 50\% Test\end{tabular} & \begin{tabular}[c]{@{}c@{}}50\% Train\\ 50\% Test\end{tabular} & \begin{tabular}[c]{@{}c@{}}50\% Train\\ 50\% Test\end{tabular} & Not used & Not used \\ \bottomrule
\end{tabular}
\caption{{\small All the experiments performed on WPP-RGBD dataset. We explored using some palpation patterns for training and others for testing to evaluate the network's ability to generalise (WPP1 to WPP8). We explored removing some patterns entirely (WPP3, WPP4, WPP7, WPP8 and WPP10). We explored training and testing on the whole dataset (WPP9 and WPP10).}}
\label{tab:wpp_experiments}
\end{table*}

\begin{table*}
\centering
\begin{threeparttable}[tb!]
\begin{tabular}{@{}ccccccccccc@{}}
\toprule
 && \multicolumn{4}{c}{MSE$^*$} && \multicolumn{4}{c}{Absolute Error$^{**}$} \\
\cmidrule{3-6} \cmidrule{8-11} && Config. I & Config. II & Config. III & Config. IV && Config. I & Config. II & Config. III & Config. IV \\
\midrule
%A 
WPP1 && 0.0662 & 0.0482 & 0.1439 & \textbf{0.0161} && \textbf{54.8} & \textbf{52.1} & 85.7 & 69.0 \\
WPP2 && 0.0470 & 0.0738 & 0.0344 & 0.0228 && 75.1 & 82.4 & 116.3 & 47.6 \\
WPP3 && 0.0590 & 0.0675 & 0.0633 & 0.1116 && 112.1 & 168.7 & 177.9 & 155.5 \\
\textbf{WPP4} && 0.0340 & 0.0617 & 0.0441 & 0.0756 && 63.8 &  112.9 & 113.5 & 61.4 \\
WPP5 && 0.1035 & 0.0310 & 0.0273 & 0.0334 && 94.5 & 131.1 & \textbf{35.6} & 121.2 \\
WPP6 && 0.0689 & 0.0358 & 0.0389 & 0.0254 && 111.8 & 63.4 & 77.4 & \textbf{34.8} \\
WPP7 && 0.0744 & 0.0625 & 0.0897 & 0.0992 && 84.8 & 136.7 & 93.9 & 94.3 \\
WPP8 && \textbf{0.0233} & 0.0534 & 0.0249 & 0.0707 && 65.4 & 73.2 & 74.7 & 90.2 \\
\textbf{WPP9} && 0.0373 & 0.0245 & \textbf{0.0072} & 0.0420 && 67.4 & 57.6 & 53.9 & 63.1 \\
WPP10 && 0.0648 & \textbf{0.0226} & 0.0136 & 0.0185 && 88.2 & 86.8 & 70.1 & 70.7 \\

\bottomrule
\end{tabular}
\begin{tablenotes}\footnotesize
\item[*] MSE in Radian${}^2$; $^{**}$ Absolute error in mm. 
\end{tablenotes}
\end{threeparttable}
\caption{{ \small Evaluation of WPP data set using CNN residual deep MP Model with AveMSE for each configuration of the WPP data set. The performance with AveED and Absolute Error for each configuration. WPP4 and WPP9 are also presented in the manuscript. The results for WPP9 show, as expected, the larger the dataset, the better performance of our deep MP. Moreover, the results of WPP4-- in which palpation path 1,4,5, are in the training set and 2,3 in the test set-- illustrate our model can generalise across different palpation path geometries. }}
\label{table:wpp_ablation}
\end{table*}

\subsection{WPP experiments}
Table \ref{table:wpp_configpos} shows the X,Y,Z positions of the Config I,II,III, and IV shown in Figure 5 of our main paper.

We performed many experiments using the WPP-RGBD dataset, with the objective of studying the effect of different train/test data splits, as well as some ablation studies, excluding certain palpation patterns. The exact structure of each experiment is reported in Table~\ref{tab:wpp_experiments}, while the results (Average MSE on the joint-space trajectory and Average Euclidean Distance on the last point of the trajectory in task space) are reported in Table~\ref{table:wpp_ablation}.

In the ablation studies (WPP3, WPP4, WPP7, WPP8 and WPP10), we removed palpation patterns 6 and 7 from the dataset since they were shorter in length and the most different among all patterns. We observed an increase in the loss values and a decrease in the performance. Both observations can be attributed to the reduced training set size.

In the experiments where we removed some palpation patterns from the training data to use them exclusively as testing data (WPP1, WPP2, WPP3, WPP4) the model demonstrated the ability to generalise to previously unseen palpation patterns.

Finally, the experiments where we used all palpation patterns both for training and for testing (WPP9 and WPP10) resulted in lower loss values and better performances. The two experiments reported in the main content of the paper are WPP4 and WPP9.

% <<<<<<< FIGURE BLOCK DIAGRAM>>>>>>>>
\begin{figure*}[tb!]
\centering
\includegraphics[width=0.7\textwidth]{figures/models_and_algorithms_fullpage.png}
\caption{{\small Structure and schematics of the models and algorithms used. The blue box contains the three types of models we developed. Two of them take as input a bottleneck layer from an encoder-decoder network which is fed the RGB image at home position, passing it through a CNN (a) or FC (b) network to predict the trajectory weights. The third instead uses a PointNet model to produce a global feature vector which is then fed into a FC (c) network, predicting the trajectory weights.\\
This is a larger version of Figure 2 in the paper}}
\label{fig:schem_dpromp}
\end{figure*}

%<<<<<<<<<<<<<>>>>>>>>>>>
\subsection{Deep Dynamic Movement Primitives (d-DMP) implementation}

In order to provide a comparison with state of the art, we implemented DMP \cite{ridge2020training} in place of ProMP for the CNN model on both RTP and WPP tasks.

One important parameter that determines the performance and computational costs of both DMP and ProMP is the number of basis functions used. They are not, however, directly comparable. For ProMP, we settled for $N_{\mathrm{bas}}=8$ and $N_{\mathrm{bas}}=10$ for RTP and WPP tasks, respectively, while we chose $N_{\mathrm{bas}}^{\mathrm{DMP}}=25$ for DMP as these parameters seemed to provide similar performances in representing the trajectories. It is evident that ProMP manages to represent the same complexity with a lower amount of basis functions, which makes deep MP easier to learn than d-DMP.

Another difference between ProMP and DMP is that, for $N_{\mathrm{joint}}$ joints, the former is fully characterised just by the weights $\mathbf{\Omega} \in \mathbb{R}^{N_{\mathrm{bas}}N_{\mathrm{joint}}}$, which is the only parameter the network has to learn, while the latter requires the weights for the forcing term $\mathbf{\Omega}^{\mathrm{DMP}} \in \mathbb{R}^{N_{\mathrm{bas}}^{\mathrm{DMP}}N_{\mathrm{joint}}}$, the goal joint positions $\mathbf{g}\in\mathbb{R}^{N_{\mathrm{joint}}}$, the initial positions $\mathbf{q}_0\in\mathbb{R}^{N_{\mathrm{joint}}}$, and the time scaling factor $\tau\in\mathbb{R}$. 

For RTP, the trajectories start always at the same position, i.e. home position, hence $\mathbf{q}_0$ is always known. Therefore, for RTP, the network must learn $\mathbf{\Omega}^{\mathrm{DMP}}$ and $\mathbf{g}$ only. On the other hand, for WPP, such information is not known, and the network must learn $\mathbf{\Omega}^{\mathrm{DMP}}$, $\mathbf{g}$ and $\mathbf{q}_0$. For all cases, we consider $\tau$ as a design parameter equal to $7.6$.

We decided to implement the loss function in weight space. For the RTP task we slightly modified the function proposed by \cite{ridge2020training}, adding a parameter $\alpha$ which regulates the relative importance of the goal residual with respect to the weights residual. From our Experiments values of $\alpha \in [100; 500]$ lead to the best results, so we adopted a value $\alpha = 100$. Hence, if $\mathbf{\Omega}^{\mathrm{DMP}}_{\mathrm{ps}}$ and $\mathbf{g}_{\mathrm{ps}}$ are the predicted parameters for forcing term weights and goals, respectively, and $\mathbf{\Omega}^{\mathrm{DMP}}_{\mathrm{gt}}$ and $\mathbf{g}_{\mathrm{gt}}$ are their corresponding ground truth values, the loss function is computed as

\begin{equation}
    L =  \mathrm{RMS} \left( \mathbf{\Omega}^{\mathrm{DMP}}_{\mathrm{gt}} - \mathbf{\Omega}^{\mathrm{DMP}}_{\mathrm{ps}} \right) + \alpha\ \mathrm{RMS} \left( \mathbf{g}_{\mathrm{gt}} - \mathbf{g}_{\mathrm{ps}} \right)
    \label{eq:loss_func}
\end{equation}

For WPP the loss function was considered as the root mean square of the difference between ground truth and predictions of the concatenation of $\mathbf{\Omega}^{\mathrm{DMP}}$, $\mathbf{g}$ and $\mathbf{q}_0$, as follows:

\begin{equation}
\begin{split}
L = \frac{1}{2} \mathrm{RMS} \Big( & \left[  (\mathbf{\Omega}^{\mathrm{DMP}}_{\mathrm{gt}})^T,(\mathbf{g}_{\mathrm{gt}})^T,(\mathbf{q}_{0,\mathrm{gt}})^T \right] + 
    \\
  -  & \left[ (\mathbf{\Omega}^{\mathrm{DMP}}_{\mathrm{ps}})^T,(\mathbf{g}_{\mathrm{ps}})^T,(\mathbf{q}_{0,\mathrm{ps}})^T \right] \Big)
  \label{eq:concat_loss}
\end{split}
\end{equation}

% <<<<<<< FIGURE >>>>>>>>

% =left bottom right top
\begin{figure*}[tb!]
\centering
\begin{subfigure}{.5\textwidth}
    \centering
    \includegraphics[width=\linewidth]{figures/appendix/1_3D_21.png}
    \caption{WPP1}
    \label{fig:WPP1}
\end{subfigure}%
\begin{subfigure}{.5\textwidth}
    \centering
    \includegraphics[width=\linewidth]{figures/appendix/2_3D_11.png}
    \caption{WPP2}
    \label{fig:WPP2}
\end{subfigure}
\begin{subfigure}{.5\textwidth}
    \centering
    \includegraphics[width=\linewidth]{figures/appendix/3_3D_15.png}
    \caption{WPP3}
    \label{fig:WPP3}
\end{subfigure}%
\begin{subfigure}{.5\textwidth}
    \centering
    \includegraphics[width=\linewidth]{figures/appendix/4_3D_18.png}
    \caption{WPP4}
    \label{fig:Experiment4}
\end{subfigure}
\begin{subfigure}{.5\textwidth}
    \centering
    \includegraphics[width=\linewidth]{figures/appendix/5_3D_21.png}
    \caption{WPP5}
    \label{fig:WPP5}
\end{subfigure}%
\begin{subfigure}{.5\textwidth}
    \centering
    \includegraphics[width=\linewidth]{figures/appendix/6_3D_19.png}
    \caption{WPP6}
    \label{fig:WPP6}
\end{subfigure}
\begin{subfigure}{.5\textwidth}
    \centering
    \includegraphics[width=\linewidth]{figures/appendix/7_3D_23.png}
    \caption{WPP7}
    \label{fig:WPP7}
\end{subfigure}%
\begin{subfigure}{.5\textwidth}
    \centering
    \includegraphics[width=\linewidth]{figures/appendix/8_3D_9.png}
    \caption{WPP8}
    \label{fig:WPP8}
\end{subfigure}
\begin{subfigure}{.5\textwidth}
    \centering
    \includegraphics[width=\linewidth]{figures/appendix/9_3D_5.png}
    \caption{WPP9}
    \label{fig:WPP9}
\end{subfigure}%
\begin{subfigure}{.5\textwidth}
    \centering
    \includegraphics[width=\linewidth]{figures/appendix/10_3D_13.png}
    \caption{WPP10}
    \label{fig:WPP10}
\end{subfigure}
\caption[short]{3D plot of the Robot trajectories generated by deep MP (dashed red line) and the corresponding ground truth (black solid line) of the Franka arm end-effector $\{WPP1, \dots, WPP10\}$. }
\end{figure*}

%<<<<<<<<<<<<<>>>>>>>>>>>

% <<<<<<<<<<<<FIGURE>>>>>>>>>..
\begin{sidewaysfigure*}[tb!]
\centering
\begin{subfigure}{.48\textwidth}
    \centering
    \includegraphics[width=\linewidth]{figures/appendix/1_traj_25_plot.png}
    \caption{WPP1}
    \label{fig:WPP1traj}
\end{subfigure}\hspace{0.5 cm}
\begin{subfigure}{.48\textwidth}
    \centering
    \includegraphics[width=\linewidth]{figures/appendix/2_traj_2_plot.png}
    \caption{WPP2}
    \label{fig:WPP2traj}
\end{subfigure}
\begin{subfigure}{.48\textwidth}
    \centering
    \includegraphics[width=\linewidth]{figures/appendix/3_traj_2_plot.png}
    \caption{WPP3}
    \label{fig:WPP3traj}
\end{subfigure}\hspace{0.5 cm}
\begin{subfigure}{.48\textwidth}
    \centering
    \includegraphics[width=\linewidth]{figures/appendix/4_traj_2_plot.png}
    \caption{WPP4}
    \label{fig:WPP4traj}
\end{subfigure}
\begin{subfigure}{.48\textwidth}
    \centering
    \includegraphics[width=\linewidth]{figures/appendix/5_traj_5_plot.png}
    \caption{WPP5}
    \label{fig:WPP5traj}
\end{subfigure}\hspace{0.5 cm}
\begin{subfigure}{.48\textwidth}
    \centering
    \includegraphics[width=\linewidth ]{figures/appendix/6_traj_8_plot.png}
    \caption{WPP6}
    \label{fig:WPP6traj}
\end{subfigure}
\begin{subfigure}{.48\textwidth}
    \centering
    \includegraphics[width=\linewidth ]{figures/appendix/7_traj_7_plot.png}
    \caption{WPP7}
    \label{fig:WPP7traj}
\end{subfigure}\hspace{0.5 cm}
\begin{subfigure}{.48\textwidth}
    \centering
    \includegraphics[width=\linewidth ]{figures/appendix/8_traj_6_plot.png}
    \caption{WPP8}
    \label{fig:WPP8traj}
\end{subfigure}
\begin{subfigure}{.48\textwidth}
    \centering
    \includegraphics[width=\linewidth]{figures/appendix/9_traj_12_plot.png}
    \caption{WPP9}
    \label{fig:WPP9traj}
\end{subfigure}\hspace{0.5 cm}
\begin{subfigure}{.48\textwidth}
    \centering
    \includegraphics[width=\linewidth]{figures/appendix/10_traj_5_plot.png}
    \caption{WPP10}
    \label{fig:WPP10traj}
\end{subfigure}
\caption[short]{Robot trajectories generated by deep MP  (dashed blue curves) and the corresponding ground truth (black curves) for 7 joints of Franka arm $\{WPP1, \dots, WPP10\}$.}
\end{sidewaysfigure*}

\bibliography{reference.bib}
\end{document}
